# Supplementary material for: supDQN: Supervised Rewarding Strategy Driven Deep Q-Network for sEMG Signal Decontamination
Source: arXiv:2405.05883 source file (2024-05-09)
Supplement: Supplementary file 1 [file supp.tex]

\begin{figure*}[!t]
    \centering
    \includegraphics[width=\textwidth]{figure_pdf/main_figure_supp_smaller_v2-compressed.pdf}
    \caption{Result of our method compared to the methods without finetuning (zoom in for best viewing). For all methods, we consider adding the edgemap from the pretrained output as an extra conditioning using ControlNet. Without this edgemap, other methods tend to lose the structure of the pretrained output. In some cases, however, an additional edgemap can overly constrain the output of a model, like in the second and fourth stylistic image pairs. Our method preserves the structure of the Stable Diffusion image, while faithfully applying the desired style. We use style guidance strength 3 and classifier guidance strength 5 for our method and set the IP-adapter scale and style-alignment scale to 0.5. }
    \label{fig:main_result_supp}
\end{figure*}
